# Supplementary material for: Code Prompting Elicits Conditional Reasoning Abilities in Text+Code LLMs
Source: arXiv:2401.10065 source file (2024-09-28)
Supplement: Supplementary file 1 [file 5-6-qualitative_analysis.tex]

Our previous experiments have focused on the accuracy of the answers. Obtaining a correct answer is correlated to a correct reasoning process. However, it is possible to obtain a correct answer despite an incorrect reasoning chain. Due to the difficulty of automatically evaluating the chain of thoughts, we perform a limited human evaluation. 
We sample ten instances from \texttt{BGQA-3} (i.e., the dataset with the most complex reasoning chains) where both text and code prompts return the correct answer and manually inspect the quality of the reasoning chains. Based on this limited sample, we observe that text prompts conduct a 100\% correct reasoning chain in only two cases, while code prompts do so in three cases. We identify two main types of errors: (\underline{1}) wrong conditional reasoning and (\underline{2}) commonsense errors. We provide examples of those in \Cref{table:qualitative_analysis}. This observation raises the question of whether the generated chain of thought \textit{is not faithful} to the internal reasoning of the model, as suggested by \citet{lyu2023faithful} or whether the model generated the right answer from a \textit{greedy} attempt to reach the closest plausible conclusion (code prompts shows a reasoning error in the last step of the CoT in three out of seven cases). We leave the analysis of faithfulness of chains of thoughts as future work.

\begin{table*}
    \centering
    \begin{tabular}{p{0.15\linewidth} | p{0.5\linewidth} | p{0.27\linewidth} }
    \toprule
         \textbf{Error Type} & \textbf{Example} & \textbf{Explanation} \\
         \midrule
         Commonsense &  We know the catfish has a harmonica, and according to Rule3 "\underline{if the catfish has something to sit on}, ... & The model believes a harmonica is something to sit on. \\
         Conditional Reasoning & \# We know the lion does not remove from the board one of the pieces of the dog, and according to Rule5 "if \underline{something becomes an enemy of the squid} but does not remove from the board one of the pieces of the dog, then it steals five points from the mosquito."
         
         \texttt{become\_enemy(lion, squid)==True}
        
         \texttt{not remove\_piece(lion, dog)==True}
        
         \texttt{steal\_points(lion,mosquito,5)=rule5(lion)}
        
         \texttt{steal\_points(lion, mosquito, 5)==True} & We do not know ~\texttt{become\_enemy(lion, squid) == True}, but if we assume this, we reach the question variable, so we get an answer to the question. \\
         \bottomrule
    \end{tabular}
    \caption{Examples of reasoning errors on correct instances by text and code prompts. Underline text is the cause of the error.}
    \label{table:qualitative_analysis}
\end{table*}
