# Supplementary material for: Code Prompting Elicits Conditional Reasoning Abilities in Text+Code LLMs
Source: arXiv:2401.10065 source file (2024-09-28)
Supplement: Supplementary file 2 [file boardgameqa_data_creation.tex]

This dataset is created by first generating a formal theory that represents the state of a boardgame and then, translates that theory into natural language. A theory is composed by facts, rules, and a question. 

\begin{displayquote}
\textbf{Facts}:

\quad	(squirrel, remove, sheep)\\
\quad	(zander, knock, sheep)

\textbf{Rules}:

 \quad R1: (squirrel, remove, sheep) AND\\ \quad (zander, knock, sheep) =>\\ \quad (sheep, remove, whale)
\end{displayquote}

This formal theory is later transformed into the (final) natural language instance:

\begin{displayquote}
A few players are playing a boardgame. The current state of the game is as follows. The squirrel removes from the board one of the pieces of the sheep. The zander knocks down the fortress of the sheep. And the rules of the game are as follows. Rule1: If the squirrel removes one of the pieces of the sheep and the zander knocks down the fortress of the sheep, then the sheep removes one of the pieces of the whale. Based on the game state and the rules and preferences, does the sheep remove from the board one of the pieces of the whale?
\end{displayquote}
