# Supplementary material for: Code Prompting Elicits Conditional Reasoning Abilities in Text+Code LLMs
Source: arXiv:2401.10065 source file (2024-09-28)
Supplement: Supplementary file 3 [file pipeline.tex]

Our proposed code prompting comprises 2 steps: translating the natural language problem instance into code and prompting the LLM with that code to generate a natural language answer. In the early stages of our work, we tried to generate the code and the final answer in one inference step. However, this was too complex for GPT 3.5. We often observed that the translation into code was not 100\% finished (i.e., after translating half of the document, the model stopped the translation and tried to answer the question). When we divided the task into two (i.e., translating into code and prompting the LLM with the code to generate the answer to the question), the problem of incomplete code generation disappeared.
